# Supplementary material for: Integrating behavioral experimental findings into dynamical models to inform social change interventions
Source: arXiv:2405.13224 source file (2026-04-22)
Supplement: Supplementary file 1 [file energy_policy_survey.pdf]

Start

# *CCS Policies- Conjoint Experiment*

**Thank you for participating in this study which is funded by University of Zurich.**

Through the brief survey that follows, your answers will be helpful in assessing the role of policy design features in shaping support for carbon capture and storage (often abbreviated as "CCS") policies.

**What will happen in this study?**

Your participation in this study will involve completing one survey. We anticipate that your involvement will require about 20 minutes. However, you have 1 hour to complete it, so you do not need to rush.

**Are there any potential risks in taking part in this study?**

There is no risk in participating in this study. Participation in this study is completely voluntary. You are free to decline to participate and to end participation at any time for any reason.

**What happens to the research data provided?**

All of your responses will be confidential and only the researchers involved in this study and those responsible for research oversight will have access to the information you provide.

**Will the research be published?**

The research results will be written up and published in a peer-reviewed academic journal on a strictly anonymous basis. No confidential data will be included in the data analysis or in the publication of the results.

**Who has reviewed this project?**

This study is being conducted by Radu Tanase, Manuel Mariani and Tulasi Agnihotram from University of Zurich. If you have any questions about this study, you may contact radu.tanase@business.uzh.ch

**IMPORTANR NOTICE:**

You must be at least 18 years of age to participate in this study.

Next

Consent

Are you willing to give consent to particiapet in this study?

Consent=1 ◯ Yes

Consent=2 ◯ No

Back | Next

0% 100%

Intro

## Welcome to the survey!

This is a conjoint study where we will ask you to make repeated choices between different policies regarding the scaling up of carbon capture and storage technologies (CCS).

We will first ask you to read a short text with basic information about CCS. Then, we will present the attributes that describe the policies for scaling up CCS. Once you have familiarised yourself with the topic, we will repeatedly show you three different policy scenarios and ask you to choose which one you would prefer. If you think you wouldn't prefer any, please **feel free to choose the None** option.

At the end of the survey, we will ask you some questions about your demographics.

Back Next

0% 100%

Info

## Information on CCS (carbon capture and storage technologies)

Carbon capture and storage (CCS) is a set of technologies aimed at capturing, transporting, and storing carbon dioxide (CO2) emitted from industrial facilities and power plants that use fossil fuels like coal and natural gas. CO2 emissions are one of the major contributors to climate change. The goal of CCS is to prevent CO2 from reaching the atmosphere by injecting it in suitable underground geological formations - depleted oil and gas fields and deep saline formations - for permanent storage.

This is an attention check: In order to prove that you are reading the instructions, please do not answer the question about climate change in the following screen. Instead, click on the button below it to continue to the next screen.

Some scientific studies promote CCS as a prospective solution to climate change, as it could significantly contribute to the reduction of CO2 emissions, while other studies emphasize that CCS is a very costly technology and there is a need to investigate its potential risks in order to ensure that its deployment would not have an adverse impact on people and the environment. Political discussions currently focus on how to regulate and implement the use of CCS.

In the following, we will sketch out some scenarios for a scale-up of CCS. Please take a look at these scenarios and evaluate them. If you don't agree with any of the scenarios, please select None when asked which one you would support.

Back Next

0% 100%

Attention1

Before entering the conjoint experiment, please let us know, do you think CCS is a good solution to the climate change challenge?

Back Next

0% 100%

Attributes

## Description of policy attributes and their levels

Please read the following lines carefully!

Don't worry: it is not necessary that you remember every detail, but in going through the following aspects, you should get a feel for what matters in a potential scale-up of CCS technologies.

The below mentioned policy scenarios each consist of 6 aspects:

1. **Policy type**: Which policies should be implemented to promote CCS?

a) A ban on the construction of new fossil fuel power plants without CCS in your state: According to this policy, no new coal- or gas-fired power stations can be built in your state without including CCS.

b) Government subsidies for CCS in your state: Your state government could subsidize CCS projects. This would make deployment of the technology more economically attractive.

c) Increase in taxes on fossil fuel power generation without CCS in your state: Such a policy would make fossil fuel power generation with no CCS more expensive.

2. **Policy cost**: All policies to scale up CCS would produce some costs for American consumers. However, the exact amount depends on many factors, such as the concrete policy calibration, economic conditions, etc. Estimates for a scale-up policy currently range between costs of US$ 4 and 19 per household (per month).

3. **Beginning of policy implementation**: When should the policy be implemented? Various scenarios include implementation in 2025, 2035, 2045 or 2055.

4. **Distance from residential areas**: CCS facilities are currently planned in many American states. Some people fear that they could negatively affect buildings and the safety of communities. Different rules regarding the required distance of CCS facilities from residential areas are currently being discussed: 2 miles / 5 miles / 10 miles / 50 miles.

5. **Policy endorsement**: Various stakeholders (e.g., Greenpeace or the U.S.-based Carbon Capture Coalition) and political parties (Democrats, Republicans) have their own opinions on policy proposals to scale up CCS.

6. **Percentage of your friends who endorse the policy scenario**: Think about your friends and imagine you could know if they endorse a policy scenario. This attribute represents the percentage of your friends, out of your total number of friends, who endorse it.

Back    Next

0% 100%

IntroCBC

We hope the information provided was sufficient to familiarise yourself with the topic. We will now start the choice task.

Here we repeatedly show you three different policy scenarios and ask you to choose which one you would prefer. If you think you wouldn't prefer any, please feel free to choose the None option.

Back Next

0% 100%

CBC_Random1

If these were your options, which of the following option would you choose?

(1 of 15)

| | | | |
|---|---|---|---|
| **Policy Type** | Ban on the construction of new fossil fuel power plants without CCS in your state. | Increase in taxes on fossil fuel power generation without CCS in your state. | Government subsidies for CCS in your state. |
| **Policy Costs (per household, per month)** | 14$ | 9$ | 4$ |
| **Begining of policy implementation** | 2045 | 2035 | 2055 |
| **Required distance to residential areas** | 50 miles | 10 miles | 5 miles |
| **Policy endorsement by** | Republican Party | Carbon Capture Coalition | Democratic Party |
| **% of your friends who endorse the policy scenario** | 23% | 76% | 98% |
| | CBC_Random1 Select | CBC_Random1 Select | CBC_Random1 Select |

NONE: I wouldn't choose any of these.

CBC_Random1

Select

Back Next

0% 100%

CBC_Random2

If these were your options, which of the following option would you choose?

(2 of 15)

| | | | |
|---|---|---|---|
| **Policy Type** | Ban on the construction of new fossil fuel power plants without CCS in your state. | Government subsidies for CCS in your state. | Increase in taxes on fossil fuel power generation without CCS in your state. |
| **Policy Costs (per household, per month)** | 19$ | 9$ | 14$ |
| **Begining of policy implementation** | 2025 | 2045 | 2055 |
| **Required distance to residential areas** | 2 miles | 10 miles | 50 miles |
| **Policy endorsement by** | Greenpeace | Democratic Party | Carbon Capture Coalition |
| **% of your friends who endorse the policy scenario** | 23% | 98% | 1% |
| | CBC_Random2 Select | CBC_Random2 Select | CBC_Random2 Select |

NONE: I wouldn't choose any of these.

CBC_Random2

Select

Back Next

0% 100%

CBC_Random3

If these were your options, which of the following option would you choose?

(3 of 15)

| | | | |
|---|---|---|---|
| **Policy Type** | Ban on the construction of new fossil fuel power plants without CCS in your state. | Increase in taxes on fossil fuel power generation without CCS in your state. | Government subsidies for CCS in your state. |
| **Policy Costs (per household, per month)** | 4$ | 4$ | 19$ |
| **Begining of policy implementation** | 2035 | 2025 | 2045 |
| **Required distance to residential areas** | 5 miles | 50 miles | 2 miles |
| **Policy endorsement by** | Carbon Capture Coalition | Republican Party | Greenpeace |
| **% of your friends who endorse the policy scenario** | 76% | 1% | 45% |
| | CBC_Random3 Select | CBC_Random3 Select | CBC_Random3 Select |

NONE: I wouldn't choose any of these.

CBC_Random3

Select

Back Next

0% 100%

CBC_Random4

If these were your options, which of the following option would you choose?

(4 of 15)

| | | | |
|---|---|---|---|
| **Policy Type** | Ban on the construction of new fossil fuel power plants without CCS in your state. | Increase in taxes on fossil fuel power generation without CCS in your state. | Increase in taxes on fossil fuel power generation without CCS in your state. |
| **Policy Costs (per household, per month)** | 14$ | 9$ | 19$ |
| **Begining of policy implementation** | 2025 | 2035 | 2055 |
| **Required distance to residential areas** | 10 miles | 5 miles | 2 miles |
| **Policy endorsement by** | Democratic Party | Greenpeace | Carbon Capture Coalition |
| **% of your friends who endorse the policy scenario** | 45% | 1% | 98% |
| | CBC_Random4 Select | CBC_Random4 Select | CBC_Random4 Select |

NONE: I wouldn't choose any of these.

CBC_Random4

Select

Back Next

0% 100%

CBC_Fixed1

If these were your options, which of the following option would you choose?

(5 of 15)

| | | | |
|---|---|---|---|
| **Policy Type** | Government subsidies for CCS in your state. | Government subsidies for CCS in your state. | Increase in taxes on fossil fuel power generation without CCS in your state. |
| **Policy Costs (per household, per month)** | 14$ | 14$ | 14$ |
| **Begining of policy implementation** | 2025 | 2025 | 2025 |
| **Required distance to residential areas** | 5 miles | 10 miles | 5 miles |
| **Policy endorsement by** | Democratic Party | Greenpeace | Carbon Capture Coalition |
| **% of your friends who endorse the policy scenario** | 23% | 76% | 45% |
| | CBC_Fixed1 Select | CBC_Fixed1 Select | CBC_Fixed1 Select |

NONE: I wouldn't choose any of these.

CBC_Fixed1

Select

Back Next

0% 100%

CBC_Random5

If these were your options, which of the following option would you choose?

(6 of 15)

| | | | |
|---|---|---|---|
| **Policy Type** | Government subsidies for CCS in your state. | Ban on the construction of new fossil fuel power plants without CCS in your state. | Government subsidies for CCS in your state. |
| **Policy Costs (per household, per month)** | 19$ | 9$ | 14$ |
| **Begining of policy implementation** | 2025 | 2035 | 2055 |
| **Required distance to residential areas** | 10 miles | 50 miles | 5 miles |
| **Policy endorsement by** | Carbon Capture Coalition | Democratic Party | Republican Party |
| **% of your friends who endorse the policy scenario** | 23% | 45% | 76% |
| | CBC_Random5 Select | CBC_Random5 Select | CBC_Random5 Select |

NONE: I wouldn't choose any of these.

CBC_Random5

Select

Back Next

0% 100%

CBC_Random6

If these were your options, which of the following option would you choose?

(7 of 15)

| | | | |
|---|---|---|---|
| **Policy Type** | Ban on the construction of new fossil fuel power plants without CCS in your state. | Increase in taxes on fossil fuel power generation without CCS in your state. | Government subsidies for CCS in your state. |
| **Policy Costs (per household, per month)** | 4$ | 19$ | 9$ |
| **Begining of policy implementation** | 2045 | 2025 | 2055 |
| **Required distance to residential areas** | 10 miles | 5 miles | 2 miles |
| **Policy endorsement by** | Greenpeace | Democratic Party | Republican Party |
| **% of your friends who endorse the policy scenario** | 98% | 45% | 76% |
| | CBC_Random6 Select | CBC_Random6 Select | CBC_Random6 Select |

NONE: I wouldn't choose any of these.

CBC_Random6

Select

Back Next

0% 100%

CBC_Random7

If these were your options, which of the following option would you choose?

(8 of 15)

| | | | |
|---|---|---|---|
| **Policy Type** | Increase in taxes on fossil fuel power generation without CCS in your state. | Increase in taxes on fossil fuel power generation without CCS in your state. | Ban on the construction of new fossil fuel power plants without CCS in your state. |
| **Policy Costs (per household, per month)** | 4$ | 14$ | 9$ |
| **Begining of policy implementation** | 2035 | 2045 | 2025 |
| **Required distance to residential areas** | 50 miles | 2 miles | 5 miles |
| **Policy endorsement by** | Republican Party | Greenpeace | Carbon Capture Coalition |
| **% of your friends who endorse the policy scenario** | 23% | 1% | 1% |
| | CBC_Random7 Select | CBC_Random7 Select | CBC_Random7 Select |

NONE: I wouldn't choose any of these.

CBC_Random7

Select

Back Next

0% 100%

CBC_Random8

If these were your options, which of the following option would you choose?

(9 of 15)

| | | | |
|---|---|---|---|
| **Policy Type** | Government subsidies for CCS in your state. | Ban on the construction of new fossil fuel power plants without CCS in your state. | Government subsidies for CCS in your state. |
| **Policy Costs (per household, per month)** | 14$ | 19$ | 4$ |
| **Begining of policy implementation** | 2045 | 2055 | 2035 |
| **Required distance to residential areas** | 2 miles | 10 miles | 5 miles |
| **Policy endorsement by** | Carbon Capture Coalition | Republican Party | Democratic Party |
| **% of your friends who endorse the policy scenario** | 76% | 45% | 23% |
| | CBC_Random8 Select | CBC_Random8 Select | CBC_Random8 Select |

NONE: I wouldn't choose any of these.

CBC_Random8

Select

Back Next

0% 100%

CBC_Fixed2

If these were your options, which of the following option would you choose?

(10 of 15)

| | | | |
|---|---|---|---|
| **Policy Type** | Government subsidies for CCS in your state. | Government subsidies for CCS in your state. | Increase in taxes on fossil fuel power generation without CCS in your state. |
| **Policy Costs (per household, per month)** | 14$ | 14$ | 14$ |
| **Begining of policy implementation** | 2025 | 2025 | 2025 |
| **Required distance to residential areas** | 5 miles | 10 miles | 5 miles |
| **Policy endorsement by** | Democratic Party | Greenpeace | Carbon Capture Coalition |
| **% of your friends who endorse the policy scenario** | 23% | 76% | 45% |
| | CBC_Fixed2 Select | CBC_Fixed2 Select | CBC_Fixed2 Select |

NONE: I wouldn't choose any of these.

CBC_Fixed2

Select

Back Next

0% 100%

CBC_Random9

If these were your options, which of the following option would you choose?

(11 of 15)

| | | | |
|---|---|---|---|
| **Policy Type** | Increase in taxes on fossil fuel power generation without CCS in your state. | Government subsidies for CCS in your state. | Ban on the construction of new fossil fuel power plants without CCS in your state. |
| **Policy Costs (per household, per month)** | 9$ | 19$ | 14$ |
| **Begining of policy implementation** | 2025 | 2055 | 2035 |
| **Required distance to residential areas** | 2 miles | 50 miles | 10 miles |
| **Policy endorsement by** | Democratic Party | Greenpeace | Republican Party |
| **% of your friends who endorse the policy scenario** | 45% | 98% | 98% |
| | CBC_Random9 Select | CBC_Random9 Select | CBC_Random9 Select |

NONE: I wouldn't choose any of these.

CBC_Random9

Select

Back Next

0% 100%

CBC_Random10

If these were your options, which of the following option would you choose?

(12 of 15)

| | | | |
|---|---|---|---|
| **Policy Type** | Ban on the construction of new fossil fuel power plants without CCS in your state. | Government subsidies for CCS in your state. | Increase in taxes on fossil fuel power generation without CCS in your state. |
| **Policy Costs (per household, per month)** | 9$ | 14$ | 4$ |
| **Begining of policy implementation** | 2035 | 2035 | 2045 |
| **Required distance to residential areas** | 2 miles | 5 miles | 50 miles |
| **Policy endorsement by** | Republican Party | Greenpeace | Carbon Capture Coalition |
| **% of your friends who endorse the policy scenario** | 1% | 23% | 76% |
| | CBC_Random10 Select | CBC_Random10 Select | CBC_Random10 Select |

NONE: I wouldn't choose any of these.

CBC_Random10

Select

Back Next

0% 100%

CBC_Random11

If these were your options, which of the following option would you choose?

(13 of 15)

| | | | |
|---|---|---|---|
| **Policy Type** | Ban on the construction of new fossil fuel power plants without CCS in your state. | Government subsidies for CCS in your state. | Increase in taxes on fossil fuel power generation without CCS in your state. |
| **Policy Costs (per household, per month)** | 14$ | 4$ | 19$ |
| **Begining of policy implementation** | 2055 | 2025 | 2045 |
| **Required distance to residential areas** | 5 miles | 50 miles | 10 miles |
| **Policy endorsement by** | Greenpeace | Greenpeace | Democratic Party |
| **% of your friends who endorse the policy scenario** | 76% | 45% | 23% |
| | CBC_Random11 elect | CBC_Random11 elect | CBC_Random11 elect |

NONE: I wouldn't choose any of these.

CBC_Random11

Select

Back Next

0% 100%

CBC_Random12

If these were your options, which of the following option would you choose?

(14 of 15)

| | | | |
|---|---|---|---|
| **Policy Type** | Government subsidies for CCS in your state. | Ban on the construction of new fossil fuel power plants without CCS in your state. | Increase in taxes on fossil fuel power generation without CCS in your state. |
| **Policy Costs (per household, per month)** | 9$ | 19$ | 4$ |
| **Begining of policy implementation** | 2025 | 2045 | 2055 |
| **Required distance to residential areas** | 50 miles | 10 miles | 2 miles |
| **Policy endorsement by** | Carbon Capture Coalition | Republican Party | Democratic Party |
| **% of your friends who endorse the policy scenario** | 1% | 45% | 98% |
| | CBC_Random12 [illegible]elect | CBC_Random12 [illegible]elect | CBC_Random12 [illegible]elect |

NONE: I wouldn't choose any of these.

CBC_Random12

Select

Back Next

0% 100%

CBC_Random13

If these were your options, which of the following option would you choose?

(15 of 15)

| | | | |
|---|---|---|---|
| **Policy Type** | Increase in taxes on fossil fuel power generation without CCS in your state. | Ban on the construction of new fossil fuel power plants without CCS in your state. | Government subsidies for CCS in your state. |
| **Policy Costs (per household, per month)** | 14$ | 4$ | 19$ |
| **Begining of policy implementation** | 2025 | 2055 | 2035 |
| **Required distance to residential areas** | 5 miles | 10 miles | 2 miles |
| **Policy endorsement by** | Republican Party | Greenpeace | Democratic Party |
| **% of your friends who endorse the policy scenario** | 23% | 1% | 76% |
| | CBC_Random13 [illegible]elect | CBC_Random13 [illegible]elect | CBC_Random13 [illegible]elect |

NONE: I wouldn't choose any of these.

CBC_Random13

Select

Back Next

0% 100%

Scale

To help us understand how you make choices, please tell us how much you agree with the following statements.

| | Strongly agree | Agree | More or less agree | Undecided | More or less disagree | Disagree | Strongly disagree |
|---|---|---|---|---|---|---|---|
| I often consult other people to help choose the best alternative available from a product class. | Scale_r3=1 ○ | Scale_r3=2 ○ | Scale_r3=3 ○ | Scale_r3=4 ○ | Scale_r3=5 ○ | Scale_r3=6 ○ | Scale_r3=7 ○ |
| If I want to be like someone, I often try to buy the same brands that they buy. | Scale_r11=1 ○ | Scale_r11=2 ○ | Scale_r11=3 ○ | Scale_r11=4 ○ | Scale_r11=5 ○ | Scale_r11=6 ○ | Scale_r11=7 ○ |
| I rarely purchase the latest fashion styles until I am sure my friends approve of them. | Scale_r5=1 ○ | Scale_r5=2 ○ | Scale_r5=3 ○ | Scale_r5=4 ○ | Scale_r5=5 ○ | Scale_r5=6 ○ | Scale_r5=7 ○ |
| I often identify with other people by purchasing the same products and brands they purchase. | Scale_r12=1 ○ | Scale_r12=2 ○ | Scale_r12=3 ○ | Scale_r12=4 ○ | Scale_r12=5 ○ | Scale_r12=6 ○ | Scale_r12=7 ○ |
| It is important that others like the products and brands I buy. | Scale_r6=1 ○ | Scale_r6=2 ○ | Scale_r6=3 ○ | Scale_r6=4 ○ | Scale_r6=5 ○ | Scale_r6=6 ○ | Scale_r6=7 ○ |
| When buying products, I generally purchase the brands that I think others will approve of. | Scale_r7=1 ○ | Scale_r7=2 ○ | Scale_r7=3 ○ | Scale_r7=4 ○ | Scale_r7=5 ○ | Scale_r7=6 ○ | Scale_r7=7 ○ |
| I frequently gather information from friends or family about a product before I buy. | Scale_r4=1 ○ | Scale_r4=2 ○ | Scale_r4=3 ○ | Scale_r4=4 ○ | Scale_r4=5 ○ | Scale_r4=6 ○ | Scale_r4=7 ○ |
| To make sure I buy the right product/brand, I often observe what others are | Scale_r1=1 ○ | Scale_r1=2 ○ | Scale_r1=3 ○ | Scale_r1=4 ○ | Scale_r1=5 ○ | Scale_r1=6 ○ | Scale_r1=7 ○ |

| | | | | | | | |
|---|---|---|---|---|---|---|---|
| buying and using. | | | | | | | |
| I like to know what brands and products make good impressions on others. | Scale_r9=1 | Scale_r9=2 | Scale_r9=3 | Scale_r9=4 | Scale_r9=5 | Scale_r9=6 | Scale_r9=7 |
| If I have little experience with a product, I often ask my friends about the product. | Scale_r2=1 | Scale_r2=2 | Scale_r2=3 | Scale_r2=4 | Scale_r2=5 | Scale_r2=6 | Scale_r2=7 |
| If other people can see me using a product, I often purchase the brand they expect me to buy. | Scale_r8=1 | Scale_r8=2 | Scale_r8=3 | Scale_r8=4 | Scale_r8=5 | Scale_r8=6 | Scale_r8=7 |
| I achieve a sense of belonging by purchasing the same products and brands that others purchase. | Scale_r10=1 | Scale_r10=2 | Scale_r10=3 | Scale_r10=4 | Scale_r10=5 | Scale_r10=6 | Scale_r10=7 |

Back Next

0% 100%

Avdsim

To help us understand how you make choices, please tell us how much you agree with the following statements.

| | Strongly agree | Agree | More or less agree | Undecided | More or less disagree | Disagree | Strongly disagree |
|---|---|---|---|---|---|---|---|
| When products or brands I like become extremely popular, I lose interest in them | Avdsim_r1=1 ◯ | Avdsim_r1=2 ◯ | Avdsim_r1=3 ◯ | Avdsim_r1=4 ◯ | Avdsim_r1=5 ◯ | Avdsim_r1=6 ◯ | Avdsim_r1=7 ◯ |
| I give up wearing fashions I've purchased once they become popular among the general public | Avdsim_r8=1 ◯ | Avdsim_r8=2 ◯ | Avdsim_r8=3 ◯ | Avdsim_r8=4 ◯ | Avdsim_r8=5 ◯ | Avdsim_r8=6 ◯ | Avdsim_r8=7 ◯ |
| Products don't seem to hold much value for me when they are purchased regularly by everyone | Avdsim_r7=1 ◯ | Avdsim_r7=2 ◯ | Avdsim_r7=3 ◯ | Avdsim_r7=4 ◯ | Avdsim_r7=5 ◯ | Avdsim_r7=6 ◯ | Avdsim_r7=7 ◯ |
| As a rule, I dislike products or brands that are customarily purchased by everyone | Avdsim_r5=1 ◯ | Avdsim_r5=2 ◯ | Avdsim_r5=3 ◯ | Avdsim_r5=4 ◯ | Avdsim_r5=5 ◯ | Avdsim_r5=6 ◯ | Avdsim_r5=7 ◯ |
| When a product I own becomes popular among the general population, I begin using it less | Avdsim_r3=1 ◯ | Avdsim_r3=2 ◯ | Avdsim_r3=3 ◯ | Avdsim_r3=4 ◯ | Avdsim_r3=5 ◯ | Avdsim_r3=6 ◯ | Avdsim_r3=7 ◯ |
| I avoid products or brands that have already been accepted and purchased by the average consumer | Avdsim_r2=1 ◯ | Avdsim_r2=2 ◯ | Avdsim_r2=3 ◯ | Avdsim_r2=4 ◯ | Avdsim_r2=5 ◯ | Avdsim_r2=6 ◯ | Avdsim_r2=7 ◯ |

| | | | | | | | |
|---|---|---|---|---|---|---|---|
| The more commonplace a product or brand is among the general population, the less interested I am in buying it | Avdsim_r6=1 ◯ | Avdsim_r6=2 ◯ | Avdsim_r6=3 ◯ | Avdsim_r6=4 ◯ | Avdsim_r6=5 ◯ | Avdsim_r6=6 ◯ | Avdsim_r6=7 ◯ |
| I often try to avoid products or brands that I know are bought by the general population | Avdsim_r4=1 ◯ | Avdsim_r4=2 ◯ | Avdsim_r4=3 ◯ | Avdsim_r4=4 ◯ | Avdsim_r4=5 ◯ | Avdsim_r4=6 ◯ | Avdsim_r4=7 ◯ |

Back Next

0% 100%

EnvScale

Please rate each of the following items from 1(not important) to 7 (supreme importance) in response to the question:

I am concerned about environmental problems because of the concequences for

| | 1 (not important) | 2 | 3 | 4 | 5 | 6 | 7 (ver |
|---|---|---|---|---|---|---|---|
| Plants | EnvScale_r1=1 | EnvScale_r1=2 | EnvScale_r1=3 | EnvScale_r1=4 | EnvScale_r1=5 | EnvScale_r1=6 | Env |
| Marine life | EnvScale_r2=1 | EnvScale_r2=2 | EnvScale_r2=3 | EnvScale_r2=4 | EnvScale_r2=5 | EnvScale_r2=6 | Env |
| Birds | EnvScale_r3=1 | EnvScale_r3=2 | EnvScale_r3=3 | EnvScale_r3=4 | EnvScale_r3=5 | EnvScale_r3=6 | Env |
| Animals | EnvScale_r4=1 | EnvScale_r4=2 | EnvScale_r4=3 | EnvScale_r4=4 | EnvScale_r4=5 | EnvScale_r4=6 | Env |
| Myself | EnvScale_r5=1 | EnvScale_r5=2 | EnvScale_r5=3 | EnvScale_r5=4 | EnvScale_r5=5 | EnvScale_r5=6 | Env |
| My health | EnvScale_r6=1 | EnvScale_r6=2 | EnvScale_r6=3 | EnvScale_r6=4 | EnvScale_r6=5 | EnvScale_r6=6 | Env |
| My lifestyle | EnvScale_r7=1 | EnvScale_r7=2 | EnvScale_r7=3 | EnvScale_r7=4 | EnvScale_r7=5 | EnvScale_r7=6 | Env |
| My future | EnvScale_r8=1 | EnvScale_r8=2 | EnvScale_r8=3 | EnvScale_r8=4 | EnvScale_r8=5 | EnvScale_r8=6 | Env |
| People in my country/community | EnvScale_r9=1 | EnvScale_r9=2 | EnvScale_r9=3 | EnvScale_r9=4 | EnvScale_r9=5 | EnvScale_r9=6 | Env |
| All people | EnvScale_r10=1 | EnvScale_r10=2 | EnvScale_r10=3 | EnvScale_r10=4 | EnvScale_r10=5 | EnvScale_r10=6 | EnvS |
| Children/My children | EnvScale_r11=1 | EnvScale_r11=2 | EnvScale_r11=3 | EnvScale_r11=4 | EnvScale_r11=5 | EnvScale_r11=6 | EnvS |
| Future generation | EnvScale_r12=1 | EnvScale_r12=2 | EnvScale_r12=3 | EnvScale_r12=4 | EnvScale_r12=5 | EnvScale_r12=6 | EnvS |

Back Next

0% 100%

Demo

Finally, please answer the following demographic questions:

Age

What is your approximate age?

Age=1 ◯ 18-24

Age=2 ◯ 25-34

Age=3 ◯ 35-44

Age=4 ◯ 45-54

Age=5 ◯ 55-64

Age=6 ◯ 65-74

Age=7 ◯ 75 or above

Age=8 ◯ Prefer not to say

gender

What is your gender?

gender=1 ◯ Male

gender=2 ◯ Female

gender=3 ◯ Other

gender=4 ◯ Prefer not to say

Education

What is the highest level of school you have completed or the highest degree you have received?

Education=1 ◯ Less than high school degree

Education=2 ◯ High school graduate (high school diploma or equivalent including GED)

Education=3 ◯ Some college but no degree

Education=4 ◯ Associate degree in college (2-year)

Education=5 ◯ Bachelor's degree in college (4-years)

Education=6 ◯ Master's degree

Education=7 ◯ Doctoral degree

Education=8 ◯ Professional degree ( JD,MD)

Education=9 ◯ Prefer not to say

subj

What was your major subject of study?

subj=1 ◯ Economics (accounting, business administration, economy)

subj=2 ◯ Humanities (literature, language, history, phylosophy)

subj=3 ◯ Science (biology, medicine, physics, mathematics, statistics, data science, engineering)

subj=4 ◯ None of the above

Income

Please indicate your approximate yearly household income before taxes. (Include total income of all adults living in your household.)

Income=1 ◯ Under $25,000

Income=2 ◯ $25,001 - $49,999

Income=3 ◯ $50,000 - $74,999

Income=4 ◯ $75,000 - $99,999

Income=5 ◯ $100,000 - $149,999

Income=6 ◯ $150,000 - $249,999

Income=7

$250,000 and over

Income=8

Prefer not to say

politcs

How would you describe your political orientation?

politcs=1

Conservative and nationalist (strongly emphasizing tradition, national aspirations and security)

politcs=2

Liberal and anti-traditional (strongly emphasizing tolerance, civil liberties, and individual freedom)

politcs=3

None of above

Socialmedia

Think of the social media platform where you are most active. Please tell us how many connections you approximately have on this platform.

Back Next

0% 100%

AttentionTerminate

Thank you for your time. Unfortunately we cannot allow you to take the survey as you have failed to follow the instructions.

0% 100%

Thanks

Thank you for participating in this survey. Your answers will help us improve our understanding how people choose when they have options to choose from.

Comments

We are always interested in your thoughts and perceptions of our study. Do you have any comments for the researchers? Any parts that were confusing or unclear? Please leave your comments below.

code

Your completion code is **88D4444F**. Please provide this code in the Prolific code box. Click on the "Submit" button below to finish the study and receive your compensation.

Back Next

0% 100%

Bye

0% 100%
