# Supplementary material for: Integrating behavioral experimental findings into dynamical models to inform social change interventions
Source: arXiv:2405.13224 source file (2026-04-22)
Supplement: Supplementary file 2 [file messaging_app_survey.pdf]

Welcome

## Welcome to the survey

In this study we aim to understand what makes new instant messaging apps attractive to consumers.

In the beginning of the survey, you will be asked to participate in a conjoint study, measuring your preference for different apps.

We will repeatedly show you three apps, which differ in terms of several attributes and ask to choose which one you would consider using instead of the app you are currently using. If you don't like any of the choices provided, please feel free to select none.

At the end of the survey, we will ask you some questions about how you make decisions and about your demographics.

Next

attcheckimg

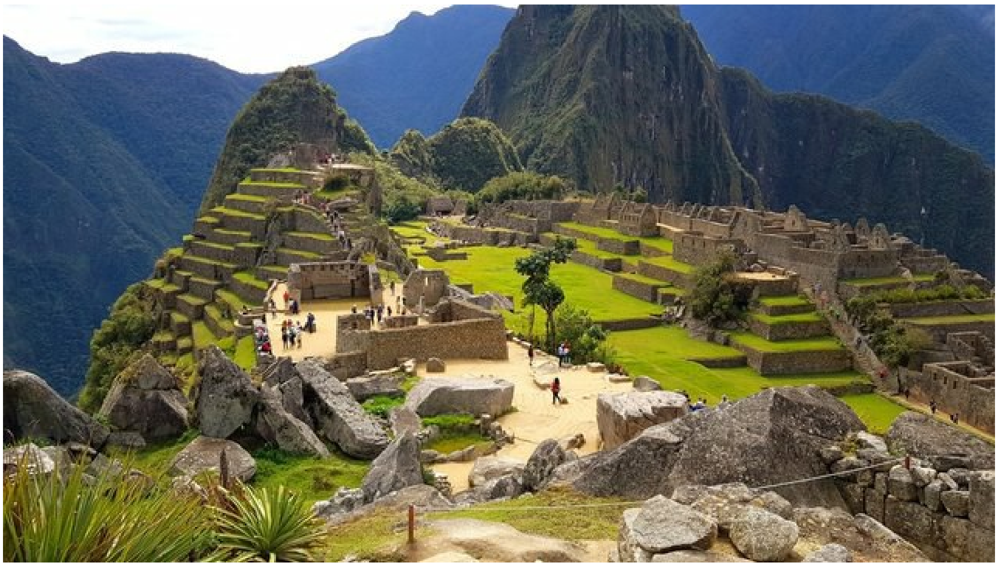

Please describe the picture in minimum 20 words.

Back Next

0% 100%

messapp

Do you currently use an instant messaging app?

messapp=1 Yes

messapp=2 No

whichapp

If yes, which one?

Back Next

0% 100%

Description

Imagine there are several new multiple instant messaging apps on the market . All apps are free and are similar to each other in all but the aspects described below. Furthermore, we ask you to imagine several of your friends are already using such an app. We will show you this information as one of the app attributes.

The apps differ in terms of the following attributes.

**Accessibility**
Instant messaging apps differ in the way you can access them. They can be:

- **Mobile only**: A mobile only app is specifically developed for smartphones and tablets. It takes full advantage of mobile device features such as push notifications, camera integration, and location services. It offers a seamless, on-the-go communication experience, but it's not accessible on desktop or web browsers.
- **Web accessible**: Web-accessible instant messaging apps expand their reach beyond mobile devices. They allow users to access their chats and conversations via web browsers on desktop computers or laptops. This versatility enables seamless transition between devices, convenient typing with a physical keyboard, and the ability to share files and links more easily on a larger screen.

**Authentication**
Authentication is important to safeguard your personal information and ensure that your conversations remain private. The apps can use one of the three levels of authentication described below, sorted by the least to the most secure:

- **Simple authentication**: Login with username and password.
- **Two-factor authentication**: Two-factor authentication (2FA) requires an additional authentication method beyond your username and password. This involves receiving a one-time verification code via SMS or email, which you must enter alongside your password to access your account.
- **Multi-factor authentication**: In addition to your username, password, and the SMS or email verification code, you must also verify your identity using a fingerprint scanner or a hardware token (a device connected to your mobile or computer).

**Customisation level**
The customization level determines how much you can personalize your messaging experience. It can take one of the following values:

- **Low**: You can adjust the basic settings, like security and notification preferences.
- **Medium**: In addition to the basic settings, you have the flexibility to shape

your chat organization, such as creating chat lists and pinning important conversations to the top.
- **High**: Additionally, you have the option to customize themes and appearance, including elements like color schemes, backgrounds, fonts used and many others.

**Video Calls**
To make the most of your video communication experience, apps focus either on One-on-one or multi-person video calls.

- **One-on-One**: The app provides a straightforward and personal video calling experience designed and optimised for one-on-one interactions. The app does not support video calls between more than two people at once.
- **Multi-person**: The app offers a versatile video calling feature, allowing you to connect with multiple participants simultaneously.

**Percentage of friends already using the app**
Imagine several of your friends use the app. This attribute shows the percentage of friends who already use this particular app. You can think about it as how many of your friends, out of all your friends are using the app. For example, if you have 10 friends and 5 of them already use the app, the percentage would be 50%.

Back Next

0% 100%

instruction

In the next questions we will repeatedly show you 3 apps which differ in terms of the attributes previously described and ask you to select which one (out of the three) you would use instead of the app you are currently using. If you don't like any of the options, please feel free to select "None".

Back Next

0% 100%

CBCmess_Random1

If these were your only options, which one would you choose to use instead of the app you are currently using?

(1 of 14)

| | | | |
|---|---|---|---|
| **Accessibility** | Mobile only | Mobile only | Web accessible |
| **Authentication** | Multi-factor authentication | Simple authentication | Two-factor authentication: |
| **Customisation level** | Medium | Low | High |
| **Video Calls** | Multi-person | One-on-One | Multi-person |
| **Percentage of friends already using the app** | 45% | 76% | 98% |
| | CBCmess_Random1 t | CBCmess_Random1 t | CBCmess_Random1 t |

None: I wouldn't choose any of these, I prefer my current instant messaging app.

CBCmess_Random1

Select

Back Next

0% 100%

CBCmess_Random2

If these were your only options, which one would you choose to use instead of the app you are currently using?

(2 of 14)

| | | | |
|---|---|---|---|
| **Accessibility** | Web accessible | Web accessible | Web accessible |
| **Authentication** | Two-factor authentication: | Multi-factor authentication | Two-factor authentication: |
| **Customisation level** | High | Low | Medium |
| **Video Calls** | One-on-One | Multi-person | Multi-person |
| **Percentage of friends already using the app** | 23% | 76% | 1% |
| | CBCmess_Random2 t | CBCmess_Random2 t | CBCmess_Random2 t |

None: I wouldn't choose any of these, I prefer my current instant messaging app.

CBCmess_Random2

Select

Back    Next

0% 100%

CBCmess_Random3

If these were your only options, which one would you choose to use instead of the app you are currently using?

(3 of 14)

| | | | |
|---|---|---|---|
| **Accessibility** | Mobile only | Web accessible | Mobile only |
| **Authentication** | Two-factor authentication: | Simple authentication | Multi-factor authentication |
| **Customisation level** | High | Low | Medium |
| **Video Calls** | Multi-person | One-on-One | One-on-One |
| **Percentage of friends already using the app** | 45% | 76% | 1% |
| | CBCmess_Random3 t | CBCmess_Random3 t | CBCmess_Random3 t |

None: I wouldn't choose any of these, I prefer my current instant messaging app.

CBCmess_Random3

Select

Back Next

0% 100%

CBCmess_Random4

If these were your only options, which one would you choose to use instead of the app you are currently using?

(4 of 14)

| | | | |
|---|---|---|---|
| **Accessibility** | Web accessible | Mobile only | Mobile only |
| **Authentication** | Simple authentication | Two-factor authentication: | Multi-factor authentication |
| **Customisation level** | Low | Medium | High |
| **Video Calls** | Multi-person | Multi-person | One-on-One |
| **Percentage of friends already using the app** | 23% | 23% | 98% |
| | CBCmess_Random4 t | CBCmess_Random4 t | CBCmess_Random4 t |

None: I wouldn't choose any of these, I prefer my current instant messaging app.

CBCmess_Random4

Select

Back Next

0% 100%

CBCmess_Fixed1

If these were your only options, which one would you choose to use instead of the app you are currently using?

(5 of 14)

| | | | |
|---|---|---|---|
| **Accessibility** | Web accessible | Mobile only | Web accessible |
| **Authentication** | Simple authentication | Multi-factor authentication | Multi-factor authentication |
| **Customisation level** | High | High | Low |
| **Video Calls** | Multi-person | Multi-person | One-on-One |
| **Percentage of friends already using the app** | 23% | 98% | 45% |
| | CBCmess_Fixed1 ect | CBCmess_Fixed1 ect | CBCmess_Fixed1 ect |

None: I wouldn't choose any of these, I prefer my current instant messaging app.

CBCmess_Fixed1

Select

Back Next

0% 100%

CBCmess_Random5

If these were your only options, which one would you choose to use instead of the app you are currently using?

(6 of 14)

| | | | |
|---|---|---|---|
| **Accessibility** | Web accessible | Web accessible | Mobile only |
| **Authentication** | Simple authentication | Multi-factor authentication | Simple authentication |
| **Customisation level** | Low | High | Medium |
| **Video Calls** | One-on-One | One-on-One | Multi-person |
| **Percentage of friends already using the app** | 1% | 45% | 76% |
| | CBCmess_Random5 t | CBCmess_Random5 t | CBCmess_Random5 t |

None: I wouldn’t choose any of these, I prefer my current instant messaging app.

CBCmess_Random5

Select

Back Next

0% 100%

CBCmess_Random6

If these were your only options, which one would you choose to use instead of the app you are currently using?

(7 of 14)

| | | | |
|---|---|---|---|
| **Accessibility** | Mobile only | Web accessible | Mobile only |
| **Authentication** | Two-factor authentication: | Simple authentication | Two-factor authentication: |
| **Customisation level** | Low | High | Medium |
| **Video Calls** | One-on-One | Multi-person | One-on-One |
| **Percentage of friends already using the app** | 1% | 98% | 23% |
| | CBCmess_Random6 t | CBCmess_Random6 t | CBCmess_Random6 t |

None: I wouldn't choose any of these, I prefer my current instant messaging app.

CBCmess_Random6

Select

Back Next

0% 100%

CBCmess_Random7

If these were your only options, which one would you choose to use instead of the app you are currently using?

(8 of 14)

| | | | |
|---|---|---|---|
| **Accessibility** | Web accessible | Mobile only | Mobile only |
| **Authentication** | Multi-factor authentication | Simple authentication | Simple authentication |
| **Customisation level** | Medium | Low | High |
| **Video Calls** | Multi-person | Multi-person | One-on-One |
| **Percentage of friends already using the app** | 76% | 45% | 23% |
| | CBCmess_Random7 t | CBCmess_Random7 t | CBCmess_Random7 t |

None: I wouldn't choose any of these, I prefer my current instant messaging app.

CBCmess_Random7

Select

Back Next

0% 100%

CBCmess_Random8

If these were your only options, which one would you choose to use instead of the app you are currently using?

(9 of 14)

| | | | |
|---|---|---|---|
| **Accessibility** | Web accessible | Mobile only | Web accessible |
| **Authentication** | Multi-factor authentication | Multi-factor authentication | Two-factor authentication: |
| **Customisation level** | Medium | Low | High |
| **Video Calls** | One-on-One | Multi-person | One-on-One |
| **Percentage of friends already using the app** | 98% | 98% | 45% |
| | CBCmess_Random8 t | CBCmess_Random8 t | CBCmess_Random8 t |

None: I wouldn’t choose any of these, I prefer my current instant messaging app.

CBCmess_Random8

Select

Back Next

0% 100%

CBCmess_Fixed2

If these were your only options, which one would you choose to use instead of the app you are currently using?

(10 of 14)

| | | | |
|---|---|---|---|
| **Accessibility** | Web accessible | Web accessible | Mobile only |
| **Authentication** | Two-factor authentication: | Simple authentication | Multi-factor authentication |
| **Customisation level** | Medium | Medium | Low |
| **Video Calls** | One-on-One | One-on-One | Multi-person |
| **Percentage of friends already using the app** | 45% | 76% | 23% |
| | CBCmess_Fixed2 ect | CBCmess_Fixed2 ect | CBCmess_Fixed2 ect |

None: I wouldn't choose any of these, I prefer my current instant messaging app.

CBCmess_Fixed2

Select

Back Next

0% 100%

CBCmess_Random9

If these were your only options, which one would you choose to use instead of the app you are currently using?

(11 of 14)

| | | | |
|---|---|---|---|
| **Accessibility** | Web accessible | Web accessible | Mobile only |
| **Authentication** | Multi-factor authentication | Simple authentication | Two-factor authentication: |
| **Customisation level** | Medium | High | Low |
| **Video Calls** | One-on-One | One-on-One | Multi-person |
| **Percentage of friends already using the app** | 23% | 45% | 1% |
| | CBCmess_Random9 t | CBCmess_Random9 t | CBCmess_Random9 t |

None: I wouldn't choose any of these, I prefer my current instant messaging app.

CBCmess_Random9

Select

Back Next

0% 100%

CBCmess_Random10

If these were your only options, which one would you choose to use instead of the app you are currently using?

(12 of 14)

| | | | |
|---|---|---|---|
| **Accessibility** | Mobile only | Web accessible | Mobile only |
| **Authentication** | Two-factor authentication: | Simple authentication | Multi-factor authentication |
| **Customisation level** | High | Medium | High |
| **Video Calls** | One-on-One | Multi-person | Multi-person |
| **Percentage of friends already using the app** | 1% | 23% | 98% |
| | CBCmess_Random10 | CBCmess_Random10 | CBCmess_Random10 |

None: I wouldn't choose any of these, I prefer my current instant messaging app.

CBCmess_Random10

Select

Back Next

0% 100%

CBCmess_Random11

If these were your only options, which one would you choose to use instead of the app you are currently using?

(13 of 14)

| | | | |
|---|---|---|---|
| **Accessibility** | Mobile only | Web accessible | Mobile only |
| **Authentication** | Two-factor authentication: | Multi-factor authentication | Simple authentication |
| **Customisation level** | Low | Low | Medium |
| **Video Calls** | One-on-One | Multi-person | One-on-One |
| **Percentage of friends already using the app** | 45% | 76% | 1% |
| | CBCmess_Random11 | CBCmess_Random11 | CBCmess_Random11 |

None: I wouldn't choose any of these, I prefer my current instant messaging app.

CBCmess_Random11

Select

Back Next

0% 100%

CBCmess_Random12

If these were your only options, which one would you choose to use instead of the app you are currently using?

(14 of 14)

| | | | |
|---|---|---|---|
| **Accessibility** | Web accessible | Web accessible | Mobile only |
| **Authentication** | Multi-factor authentication | Two-factor authentication: | Simple authentication |
| **Customisation level** | Low | Medium | Medium |
| **Video Calls** | Multi-person | Multi-person | One-on-One |
| **Percentage of friends already using the app** | 23% | 98% | 45% |
| | CBCmess_Random12 | CBCmess_Random12 | CBCmess_Random12 |

None: I wouldn't choose any of these, I prefer my current instant messaging app.

CBCmess_Random12

Select

Back Next

0% 100%

privacycheck

On a scale of 1 to 5, with 1 being 'Not Important at All' and 5 being 'Extremely Important', how would you rate the importance of security and privacy features when using instant messaging apps?

privacycheck=1 ◯ 1. Not at all important

privacycheck=2 ◯ 2.

privacycheck=3 ◯ 3.

privacycheck=4 ◯ 4.

privacycheck=5 ◯ 5. Extremely Important

Back Next

0% 100%

Scale1

To understand how you make choices, please answer the following questions.

| | Strongly disagree | Disagree | Somewhat disagree | Neither agree nor disagree | Somewhat agree | Agree | Strongly agree |
|---|---|---|---|---|---|---|---|
| I rarely purchase the latest fashion styles until I am sure my friends approve of them. | Scale1_r5=1 | Scale1_r5=2 | Scale1_r5=3 | Scale1_r5=4 | Scale1_r5=5 | Scale1_r5=6 | Scale1_r5=7 |
| I frequently gather information from friends or family about a product before I buy. | Scale1_r4=1 | Scale1_r4=2 | Scale1_r4=3 | Scale1_r4=4 | Scale1_r4=5 | Scale1_r4=6 | Scale1_r4=7 |
| I often consult other people to help choose the best alternative available from a product class. | Scale1_r3=1 | Scale1_r3=2 | Scale1_r3=3 | Scale1_r3=4 | Scale1_r3=5 | Scale1_r3=6 | Scale1_r3=7 |
| I often identify with other people by purchasing the same products and brands they purchase. | Scale1_r12=1 | Scale1_r12=2 | Scale1_r12=3 | Scale1_r12=4 | Scale1_r12=5 | Scale1_r12=6 | Scale1_r12= |
| I achieve a sense of belonging by purchasing the same products and brands that others purchase. | Scale1_r10=1 | Scale1_r10=2 | Scale1_r10=3 | Scale1_r10=4 | Scale1_r10=5 | Scale1_r10=6 | Scale1_r10= |
| When buying products, I generally purchase the brands that I think others will approve of. | Scale1_r7=1 | Scale1_r7=2 | Scale1_r7=3 | Scale1_r7=4 | Scale1_r7=5 | Scale1_r7=6 | Scale1_r7=7 |
| It is important that others like the products and brands I buy. | Scale1_r6=1 | Scale1_r6=2 | Scale1_r6=3 | Scale1_r6=4 | Scale1_r6=5 | Scale1_r6=6 | Scale1_r6=7 |
| I like to know what brands and products make good impressions on | Scale1_r9=1 | Scale1_r9=2 | Scale1_r9=3 | Scale1_r9=4 | Scale1_r9=5 | Scale1_r9=6 | Scale1_r9=7 |

others.

| | | | | | | | |
|---|---|---|---|---|---|---|---|
| If I have little experience with a product, I often ask my friends about the product. | Scale1_r2=1 | Scale1_r2=2 | Scale1_r2=3 | Scale1_r2=4 | Scale1_r2=5 | Scale1_r2=6 | Scale1_r2=7 |
| If I want to be like someone, I often try to buy the same brands that they buy. | Scale1_r11=1 | Scale1_r11=2 | Scale1_r11=3 | Scale1_r11=4 | Scale1_r11=5 | Scale1_r11=6 | Scale1_r11= |
| To make sure I buy the right product/brand, I often observe what others are buying and using. | Scale1_r1=1 | Scale1_r1=2 | Scale1_r1=3 | Scale1_r1=4 | Scale1_r1=5 | Scale1_r1=6 | Scale1_r1=7 |
| If other people can see me using a product, I often purchase the brand they expect me to buy. | Scale1_r8=1 | Scale1_r8=2 | Scale1_r8=3 | Scale1_r8=4 | Scale1_r8=5 | Scale1_r8=6 | Scale1_r8=7 |

Back    Next

0% 100%

Age

What is your approximate age?

- Age=1 ○ 18-24
- Age=2 ○ 25-34
- Age=3 ○ 35-44
- Age=4 ○ 45-54
- Age=5 ○ 55-64
- Age=6 ○ 65-74
- Age=7 ○ 75 or above
- Age=8 ○ Prefer not to say

Back Next

0% 100%

gender

What is your gender?

gender=1 ◯ Male

gender=2 ◯ Female

gender=3 ◯ Other

gender=4 ◯ Prefer not to say

Back | Next

0% 100%

Education

What is the highest level of school you have completed or the highest degree you have received?

- Education=1 ○ Less than high school degree
- Education=2 ○ High school graduate (high school diploma or equivalent including GED)
- Education=3 ○ Some college but no degree
- Education=4 ○ Associate degree in college (2-year)
- Education=5 ○ Bachelor's degree in college (4-years)
- Education=6 ○ Master's degree
- Education=7 ○ Doctoral degree
- Education=8 ○ Professional degree ( JD,MD)
- Education=9 ○ Prefer not to say

Back Next

0% 100%

subj

What was your major subject of study?

subj=1 ◯ Economics (accounting, business administration, economy)

subj=2 ◯ Humanities (literature, language, history, philosophy)

subj=3 ◯ Science (biology, medicine, physics, mathematics, statistics, data science, engineering)

subj=4 ◯ None of the above

Back Next

0% 100%

Income

Please indicate your approximate yearly household income before taxes. (Include total income of all adults living in your household.)

- Income=1 ◯ Under $25,000
- Income=2 ◯ $25,001 - $49,999
- Income=3 ◯ $50,000 - $74,999
- Income=4 ◯ $75,000 - $99,999
- Income=5 ◯ $100,000 - $149,999
- Income=6 ◯ $150,000 - $249,999
- Income=7 ◯ $250,000 and over
- Income=8 ◯ Prefer not to say

Back Next

0% 100%

id

**Thank you for participating in the survey!**

Please type in your Prolific ID so that we know you completed the survey.

Back Next

0% 100%

thoughts

We are always interested in your thoughts and perceptions of our studies. Do you have any comments for the researchers? Any parts that were confusing or unclear?

Back Next

0% 100%

Terminate

**Your completion code is C16CDTTN. Please provide this in the Prolific code box.**

0% 100%
